# Supplementary material for: Study of dynamical heterogeneities in aging colloidal nanoclay suspensions
Source: arXiv:1610.04431 ancillary file (2016-10-14)
Supplement: Supplementary file 1 [file Supporting_Information.pdf]

**Supporting Information**

Title**:** *Study of dynamical heterogeneities in aging colloidal nanoclay suspensions*

**Note on determination of $\tau_1$:**

The relaxation time ($\tau_1$) of a spherical particle is related to its diffusion coefficient $D_1$ by: $\tau_1 = 1/D_1q^2$ where q is the scattering wave vector. According to the Stokes-Einstein (SE) relation, $D_1 = k_BT/6\pi\eta r_h$ for a dilute suspension of spherical monodisperse particles, where $k_B$, T, $\eta$ and $r_h$ are the Boltzmann constant, temperature, viscosity of the medium and hydrodynamic radius of the particle respectively. Since the Laponite platelet is a disk-shaped particle with diameter d=25-30nm and thickness h=1nm, its equivalent spherical diameter (ESD) ($d_s$) is given by the Jennings-Parslow relation [1]

$$d_s = d\left(\frac{3\tan^{-1}\left(\sqrt{\left(\frac{d}{h}\right)^2-1}\right)}{2\sqrt{\left(\frac{d}{h}\right)^2-1}}\right)^{1/2}$$

From the above relation, the effective spherical diameter of the Laponite particle is, $d_s$= 7.5-8.3 nm. $\tau_1$ is related to spherical particle radius ($r_h=d_s/2$) from SE relation

$$\tau_1 = \frac{1}{D_1q^2} = \frac{6\pi\eta r_h}{k_BTq^2}$$

For q = 0.0223 $nm^{-1}$, $\eta$=0.89 mPa.s at T=25°C gives us $\tau_1 \approx 30 - 34$ μsec. This $\tau_1$ value is fixed while fitting the experimental data with the Eq.3 and Eq.8 shown in the manuscript.

Table S1: Fitting parameters obtained by fitting Eq.3 (given in main text) to the data shown in Fig.1 with increasing $t_w$.

| $t_w(h)$ | *a* (±0.003) | $\tau_\alpha=(\tau_{ww}/\beta)\Gamma(1/\beta)$ (μs) | β (±0.01) |
|---|---|---|---|
| **1.53** | 0.036 | 1513.8±11.8 | 0.94 |
| **2.03** | 0.037 | 1820.6±13.7 | 0.93 |
| **3.75** | 0.061 | 2545.1±24.6 | 0.92 |
| **5.27** | 0.028 | 3939.5±25.3 | 0.83 |
| **6.43** | 0.022 | 5684.8±33.1 | 0.78 |
| **7.7** | 0.025 | 8886.5±61.4 | 0.73 |
| **9.4** | 0.022 | 17453.1±116.9 | 0.67 |
| **10.22** | 0.02 | 27131.7±253.4 | 0.63 |
| **11.22** | 0.002 | 46977.4±589.1 | 0.53 |
| **12.47** | 0.009 | 101532.2±594.5 | 0.52 |
| **13.4** | 0.007 | 239309.1±2877.6 | 0.45 |
| **14.58** | 0.018 | 662571. 9±3277.1 | 0.40 |
| **16.6** | 0.006 | $2.2\times10^6$±7814.6 | 0.37 |

Table S2: Fitting parameters obtained by fitting the data shown in Fig.3 to Eq.8 (shown in main text) with increasing $t_w$. The fixed parameters in the equation are $\tau_1$=30 μs and VFT parameters, $D$=6.82±0.5, $t_\infty$=31.3±1.3 h, $\tau_o$=1060±65 μs.

| $t_w(h)$ (±0.2) | *a* (±0.003) | β (±0.01) |
|---|---|---|
| **1.53** | 0.042 | 0.95 |
| **3.75** | 0.041 | 0.90 |
| **6.4** | 0.034 | 0.79 |
| **9.4** | 0.019 | 0.66 |
| **11.2** | 0.01 | 0.52 |
| **13.4** | 0.012 | 0.48 |
| **14.58** | 0.004 | 0.42 |
| **16.6** | 0.009 | 0.38 |

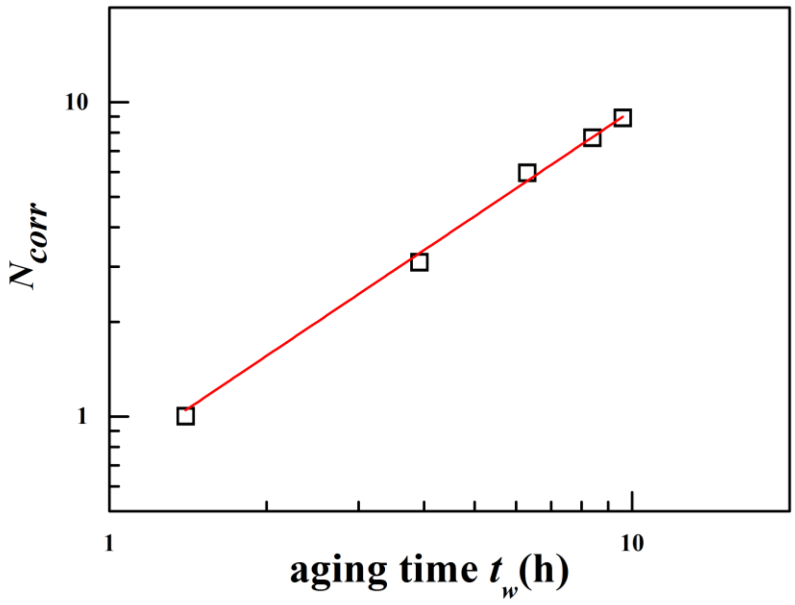


Fig.S1: Growth of number of correlated particles ($N_{corr}$) deduced at scattering angle $\theta=60^o$ as Laponite-PS system aging time ($t_w$) increases towards the non-ergodic transition. Solid line is the power law fit of the form $N_{corr}=B(t_w)^\gamma$ with $B$=0.72±0.1 and exponent $\gamma$=1.12±0.06.

## References

1. B.R. Jennings and K. Parslow, Proc. R. Soc. London A, **419,** 137 (1988).
